# Supplementary material for: UniHENN: Designing Faster and More Versatile Homomorphic Encryption-based CNNs without im2col
Source: arXiv:2402.03060 source file (2024-08-25)
Supplement: Supplementary file 1 [file 8_Appendix.tex]

\section*{Appendix}
\setcounter{figure}{0}

\subsection{ddd}
\noindent

\hyunmin{I modified the proof. If stride =1, padding = 10, kernel = 2, the lemma2 is not satisfied. So, split the case where if s=1 or not, and write the statement in the paper.}
\newtheorem{theorem}{Theorem}
\newtheorem{lemma}[theorem]{Lemma}
\begin{lemma}
\label{lemma_pooling}
Let $I, O$ be an input size and output size of the pooling layer. Then, $O \leq I$.
\end{lemma}

\begin{proof}
If the kernel size of the pooling is one than the equality is satisfied. And, the other case, the inequality is satisfied.
\end{proof}

\begin{lemma}
Let $IW \times IH$ be the input size and $N$ be the number of total convolutional layers and $OW_{i} \times OH_{i}$ be the size of the output of the $i$th convolutional layers. Then, $OW_{i} \leq IW$ and $OH_{i} \leq IH$ where padding size $(p^{l}_{i}, p^{r}_{i})$ and kernel size $(k^{l}_{i}, k^{r}_{i})$ satisfies $2\times p^{l}_{i} \leq k^{l}_{i}$, $2\times p^{r}_{i} \leq k^{r}_{i}$ for all $i \in [1, S]$.
\end{lemma}

\begin{proof}
Since by \textbf{Lemma}~\ref{lemma_pooling}, without loss of generality we do not consider the pooling layer.
For all $i$ where $1 \leq i \leq S$, assume that $(IW_i, IH_i)$ and $(OW_i, OH_i)$ be the input and output of the $i$th convolutional layers.
for all $i \in [1, S]$,
$OW_i \leq IW$ and $OH_i \leq IH$ because 
\begin{align}\notag  
OW_i = \left[ \frac{IW_{i} - k^{l}_{i} + 2\times p^{l}_{i}}{s^{l}_{i}} \right]
\end{align}\notag
and \\
\begin{align}
OH_i = \left[ \frac{IH_{i} - k^{r}_{i} + 2\times p^{r}_{i}}{s^{r}_{i}} \right]
\end{align}

Since $s^{l}_{i}, s^{r}_{i} \geq 1$, 
\begin{align}  
OW_i \leq \left[ \frac{IW_{i} - k^{l}_{i} + 2\times p^{l}_{i}}{s^{l}_{i}} \right] \\
\leq
\left[ IW_{i} - k^{l}_{i} + 2\times p^{l}_{i} \right] 
\end{align} 
and \\
\begin{align}
OH_i \leq \left[ \frac{IH_{i} - k^{r}_{i} + 2\times p^{r}_{i}}{s^{r}_{i}} \right] \\
\leq \left[ IH_{i} - k^{r}_{i} + 2\times p^{r}_{i} \right]
\end{align}

Since $2\times p^{l}_{i} \leq k^{l}_{i}$, $2\times p^{r}_{i} \leq k^{r}_{i}$ for all $i \in [1, S]$ by the condition of the statement,

\begin{align}  
OW_i \leq \left[ IW_{i} - k^{l}_{i} + 2\times p^{l}_{i} \right]
\leq 
IW_{i}
\end{align} 
and \\
\begin{align}
OH_i \leq \left[ IH_{i} - k^{r}_{i} + 2\times p^{r}_{i} \right]
\leq IH_{i} 
\end{align}

Thus, for all $i$, $OW_i \leq IW_{i}$, and $OH_i \leq IH_{i}$.
It means that $IH_{S} \leq IH$ and $OH_{S} \leq OH$.
\end{proof}
